# Supplementary material for: Hypocoercivity of Piecewise Deterministic Markov Process-Monte Carlo
Source: arXiv:1808.08592 source file (2021-08-02)
Supplement: Supplementary file 1 [file appendix.tex]

\section{About some domains...}
\subsection{DMS assumptions}
In this section, we consider an operator $(\bmcl*,\domain(\bmcl))$ on a Hilbert space $\msh$ satisfying the following assumption. 
\begin{assumption}
\label{as:DMS_generator}
  $(\bmcl,\domain(\bmcl))$ is a densily defined closed operator  and $\domain(\bmcl) = \domain(\bmcl^{*})$ on $\msh$. 
\end{assumption}
Note that the last condition is automatically satisfied by \cite[Proposition 5.1.10] {pedersen1995analysis} if
$\bmcl$ is normal,
\ie~$\bmcl \bmcl^* = \bmcl^* \bmcl$. Under
**** we let $\bmcs$ and $\bmct$ be the
$\Lmu$-symmetric and $\Lmu$-skew-symmetric parts of a generator
$\bmcl$, with common domain $\domain(\bmcs) = \domain(\bmct)= \domain(\bmcl)$ that is
\begin{equation}
  \label{eq:def_calS_calT-bar}
\bmcs = \frac{\bmcl+\bmcl^*}{2}  \quad \text{and} \quad \bmct = \frac{\bmcl-\bmcl^*}{2} \eqsp,
\end{equation}
\begin{assumption}
  \label{as:tpiv}
  The operator $(\bmct \Piv,\domain(\bmct \Piv))$ is a closable densily defined operator. 
\end{assumption}
      \begin{lemma}
        % \label{lem:bounded_A}
        \label{lemma:op norms_closed}
        Assume \Cref{as:DMS_generator} and \Cref{as:tpiv}. Then,

        $\left( m_2 + (\bmct \Piv)^* (\bmct \Piv) \right)^{-1}$ and $\mca$ are  bounded operators on $\mrl^2(\mu)$. In addition $\mca$ satisfies
        \begin{equation}
	\normopmu{ \calA}  \le  1/ (2 m_2^{\half}) \eqsp, \qquad \normopmu{ \bmct \calA } \le 1 \eqsp,\qquad  \range(\mca) \subset \domain(\mcs) \cap \domain(\mct) \eqsp.
      \end{equation}
      \alain{to show the last statement}
    \end{lemma}
    \begin{proof}
      The proof is postponed to... 
    \end{proof}

 and define the operator $\calA$ as follows,
\begin{equation}
\label{eq:defcalA-bar}
	\calA = \left( m_2 \Id + (\bmct \Piv)^* (\bmct \Piv) \right)^{-1} (-\bmct \Piv)^*\eqsp,
      \end{equation}
      where $\Piv$ is given by \eqref{eq:def_piv} and $m_2$ by \eqref{eq:def_m_2}.
The main result of \cite{Dolbeault15} can be formulated under the following abstract assumption and the proof of our main theorem relies on sharp estimates of the constants involved.
\begin{assumption}[DMS abstract conditions] \label{as:DMSabstrac-bar}
  Assume that  there exists a core $\core \subset \domain(\mcl)$ for $\mcl$ such that  
\begin{enumerate}
\item \label{item:DMS-micro_b} there exists $\lambda_v>0$ satisfying for any $\varphi \in \core$
\begin{equation}
-\psmu{  \bmcs \varphi}{ \varphi} \geq  \lambda_v m_2^{\half} \normmu{ (\Id-\Piv) \varphi }^2 \eqsp;
\end{equation}
\item \label{item:DMS-macro_b} there exists $\lambda_x\in\ooint{0,1}$ satisfying for any $\varphi \in \core$
  \begin{equation}
    \label{eq:DMS_macro_b}
-\psmu{ \calA\bmct\Piv\varphi}{\varphi} \ge \lambda_x \normmu{ \Piv \varphi }^2 \eqsp;
\end{equation}
\item \label{item:DMS-RSandRT_b} there exist $R_0 \geq 0$ satisfying for any $\varphi \in \core$
  \begin{equation*}
    \abs{\psmu{ \calA\bmct(I-\Piv)\varphi}{\varphi}+\psmu{ \calA\bmcs\varphi}{\varphi}}\leq R_0\normmu{(\Id-\Piv )\varphi} \normmu{\Piv \varphi} \eqsp;
  \end{equation*}
%  \todo{CA: really I think we can have one constant only and combine the two terms--one constant less at this stage :)}
% \begin{equation}
% \begin{aligned}
% \vert\lang \calA \bmct (\Id-\Piv) \varphi, \varphi } \vert &\leq R_{\bmct} \| (\Id-\Piv) \varphi \| \| \Piv \varphi \|, \\
% \vert \lang \calA \bmcs \varphi, \varphi } \vert &\leq  R_{\bmcs} \| (\Id-\Piv) \varphi \| \| \Piv \varphi \|.
% \end{aligned}
% \end{equation}
% {\color{red} 
% there exist $0<R_0< \infty$ such that 
% \begin{equation}
% \vert\lang \calA \bmct (\Id-\Piv) \varphi, \varphi } + \lang \calA \bmcs \varphi, \varphi } \vert \leq R_0 \| (\Id-\Piv) \varphi \| \| \Piv \varphi \|.
% \end{equation}
\item \label{item:DMS-proj-bar} $\Piv \bmct \Piv =0$ and $\range(\Piv) \subset \kernel(\mcs)$.
\end{enumerate}
\end{assumption}

%%% Local Variables:
%%% mode: latex
%%% TeX-master: "pdmp"
%%% End:
